# Supplementary material for: Revisiting Anomaly Detection in ICS: Aimed at Segregation of Attacks and Faults
Source: arXiv:2005.00325 source file (2020-04-25)
Supplement: Supplementary file 1 [file appendix.tex]

\appendix

% Table: Attack Detection Performance
\begin{table*}[!htb]
\begin{center}
\caption{Executed Attacks on SWaT Testbed from reference~\cite{sridhar_dataset_paper}}
\label{tbl:executed_attack_table}
\begin{adjustbox}{max width=2\textwidth,max height=\textheight,max totalsize={2\textwidth}{\textheight}}
%\begin{longtable}{|c | c | c | c | c | c |c |}
\begin{tabularx}{\textwidth}{|X | X | X | X | X | p{2.5cm} |p{2.5cm}| } 
 \hline
 
Attack Sequence Number &	Start Time	& 	End Time &	Attack Point	& Start State &	Attack	&	Expected Impact or Attacker Intent \\
\hline

1 &	28/12/2015 10:29:14	&		10:44:53 &	MV-101 &	MV-101 is closed	& Open MV-101	&	Tank overflow \\
\hline

2 &	28/12/2015 10:51:08	&	10:58:30 &	P-102 &	P-101 is on where as P-102 is off &	Turn on P-102 &	Pipe bursts \\
\hline

3	& 28/12/2015 11:22:00 & 	11:28:22 &	LIT-101	& Water level between L and H	& Increase by 1 mm every second	&	Tank Underflow; Damage P-101 	\\
\hline

7	& 28/12/2015 12:08:25	&	12:15:33	&	LIT-301	& Water level between L and H	& Water level increased above HH	&	Stop of inflow; Tank underflow; Damage P-301	 \\
\hline

8	& 28/12/2015 13:10:10	&	13:26:13	&	DPIT-301 &	Value of DPIT is <40kpa	& Set value of DPIT as >40kpa	&	Backwash process is started again and again; Normal operation stops; Decrease in water level of tank 401. Increase in water level of tank 301	 \\
\hline

10	& 28/12/2015 14:16:20	&	14:19:00	&	FIT-401	& Value of FIT-401 above 1	& Set value of FIT-401 as <0.7	&	UV shutdown; P-501 turns off; 	UV did not shutdown; P-501 did not turn off  \\
\hline

11	& 28/12/2015 14:19:00	&	14:28:20	&	FIT-401	& Value of FIT-401 above 1	& Set value of FIT-401 as 0	&	UV shutdown; P-501 turns off  \\
\hline

13 & 	29/12/2015 11:11:25	& 		11:15:17& 	MV-304& 	MV-304 is open& 	Close MV-304& 		Halt of stage 3 because change in the backwash process \\
\hline

14	&  29/12/2015 11:35:40	& 	11:42:50 & 	Mv-303 & 	MV-303 is closed & 	Do not let MV-303 open	& 	Halt of stage 3 because change in the backwash process \\
\hline

16	& 29/12/2015 11:57:25	&	12:02:00	&	LIT-301	& Water level between L and H	& Decrease water level by 1mm each second	&	Tank Overflow 	\\
\hline

17 &	29/12/2015 14:38:12	&		14:50:08 &	MV-303 &	MV-303 is Closed	& Do not let MV-303 open	&	Halt of stage 3 because change in the backwash process \\
\hline

21	& 29/12/2015 18:30:00	&	18:42:00	&	MV-101, LIT-101 &	MV-101 is open; LIT-101 between L and H	& Keep MV-101 on continuously; Value of LIT-101 set as 700 mm	&	Tank overflow 	\\
\hline

22  &	29/12/2015 22:55:18	&		23:03:00  &	UV-401, AIT-502, P-501 &	UV-01 is on; AIT-502 is <150; P-501 is open &	Stop UV-401; Value of AIT502 set as 150; Force P-501 to remain on	&	Possible damage to RO \\
\hline

25	& 30/12/2015 10:01:50	&	10:12:01	&	LIT-401, P-401 &	Value of LIT-401 <1000; P-402 is on	& Set value of LIT-401 as 1000; P402 is kept on	&	Tank underflow \\
\hline

26	& 30/12/2015 17:04:56	&	17:29:00	&	P-101, LIT-301 &	P-101 is off; P-102 is on; LIT-301 is between L and H	& P-101 is turned on continuously; Set value of LIT-301 as 801 mm	&	Tank 101 underflow; Tank 301 overflow	\\
\hline

27	& 31/12/2015 01:17:08	&	01:45:18	&	P-302, LIT-401 &	P302 is on, LIT401 Is  between L and H	& Keep P-302 on continuously; Value of  LIT401 set as 600 mm till 1:26:01	&	Tank overflow	\\
\hline

30	& 31/12/2015 15:47:40	&	16:07:10	&	LIT-101, P-101, MV-201	& P-101 is off; MV-101 is off; MV-201 is off; LIT-101 is between L and H;  LIT-301 is between L and H	&  Turn P-101 on continuously; Turn MV-101 on continuously; Set value of LIT-101 as 700 mm; P-102 started itself because LIT301 level became low	& 	Tank 101 underflow; Tank 301 overflow 	\\
\hline

31	& 31/12/2015 22:05:34	&	22:11:40	&	LIT-401	& Water level between L and H	& Set LIT-401 to less than L	&	Tank overflow	\\
\hline

32	& 1/01/2016 10:36:00	&	10:46:00	&	LIT-301	& Water level between L and H	& Set LIT-301 to above HH	&	Tank underflow; Damage P-302 	\\
\hline

33	& 1/01/2016 14:21:12	&	14:28:35	&	LIT-101	& Water level between L and H	& Set LIT-101 to above H	&	Tank underflow; Damage P-101	\\
\hline

35 &	1/01/2016 17:18:56	&		17:26:56 &	P-101; P-102 &	P-101 is on; P-102 is off &	Turn P-101 off; Keep P-102 off	&	Stops outflow \\
\hline

36	& 1/01/2016 22:16:01	&	22:25:00	&	LIT-101	& Water level between L and H	& Set LIT-101 to less than LL	&	Tank overflow	 \\
\hline

39	& 2/01/2015 11:43:48	&	11:50:28	&	FIT-401, AIT-502	& In Normal Range	& Set value of FIT-401 as 0.5; Set value of AIT-502 as 140 mV	&	UV will shut down and water will go to RO	UV did not shutdown  \\
\hline

40	& 2/01/2015 11:51:42	&	11:56:38	&	FIT-401 &	In Normal Range	& Set value of FIT-401 as 0	&	UV will shut down and water will go to RO	P-402 did not close, both should be interlinked  \\
\hline

41	& 2/01/2015 13:13:02	&	13:40:56	&	LIT-301	& Water level between L and H	& decrease value by 0.5 mm per second	&	Tank overflow	Rate of decrease in water level reduced after 1:33:25 PM \\ [1ex] 
 \hline
\end{tabularx}
%\end{longtable}
\end{adjustbox}
\end{center}
\end{table*}
